# Supplementary material for: Bayesian Constraint Inference from User Demonstrations Based on Margin-Respecting Preference Models
Source: arXiv:2403.02431 source file (2024-03-04)
Supplement: Supplementary file 1 [file appendix.tex]

\section*{Appendix}

\section{Simulation Details}
\subsection{Preference-Based Inverse Reinforcement Learning}\label{sec:birl}

The following algorithm was the baseline used in the experiments for the point mass and FetchReach environment comparisons.  
\begin{algorithm}[H]
\caption{Feature-Based Bayesian Constraint Inference}\label{alg:feat_inf}
\begin{algorithmic}[1]
\State \textbf{Parameters:} Number of iterations $K$, sampling frequent $f_r$
\State Randomly sample: penalty weight $\mathbf{w}_{pen}\in\mathbb{R}^f$
%\State $chain_{\mathbf{{r}}_p}[0]=\mathbf{{r}}_p$
%\State Compute $Q^{*}$ on $M_{\mathbf{{r}}_p}$
\For{$i=1,\ldots,K$ }
\State Randomly sample feature $j$ from $\{1,\ldots,f\}$
\State Set $\mathbf{w}_{pen}'[j]= \mathbf{w}_{pen}[j]+\mathcal{N}(0,\sigma)$
\State Compute Likelihood using~(\ref{eq:likeli_fn})
\If{$\log\mathcal{L}(\mathbf{w}_{pen}')\geq \log\mathcal{L}(\mathbf{w}_{pen})$}
\State Set $\mathbf{w}_{pen}=\mathbf{w}_{pen}'$
\Else
\State Set $\mathbf{w}_{pen}=\mathbf{w}_{pen}'$ w.p. $\mathcal{L}(\mathbf{w}_{pen}')/\mathcal{L}(\mathbf{w}_{pen})$
\EndIf
\EndFor
\State \textbf{Return} ${\mathbf{{w}}_{pen}}$
\end{algorithmic}
\end{algorithm}

The original policies in the environment are obtained using a SAC policy~\cite{haarnoja2018soft}. The hyperparameters of the policy training can be seen in the Table~\ref{table:SAC_params}. For the HalfCheetah and Ant s a total of $600$ episodes were used, each of maximum length of $1000$. In the fist $40$ episodes action were chosen randomly to enhance exploration.

\begin{table}[H]
\caption{Hyperparameters of SAC training.}
\centering
\begin{tabular}{cccccc}
\thickhline
 \multicolumn{3}{c}{Hyperparameter} & \multicolumn{3}{c}{Value}\\ \cmidrule(lr){1-3} \cmidrule(lr){4-6}
 %\thickhline
   & value learning rate &  &  & $3\cdot 10^{-4}$ &  \\ 
 & q learning rate &  &  & $3\cdot 10^{-4}$ &  \\ 
   &policy learning rate &  &  & $3\cdot 10^{-4}$ &  \\ 
  & batch size &  &  & $128$ &  \\ 
    & hidden dimension &  &  & $256$ &  \\ 
      & buffer size &  &  & $80000$ &  \\  
 \thickhline
\end{tabular}
\label{table:SAC_params}
\end{table}

\subsection{Point Mass and FetchReach Environment}

\subsection{HalfCheetah and Ant Environments}

\begin{Large}
\begin{center}
    NOTES (TO BE DELETED)
\end{center}
\end{Large}

\begin{itemize}
\item Uncertainty in preferences
\item \textcolor{green}{include dynamics in constraint estimation}
\item \textcolor{green}{and in inverse RL in general}

% \item \texttt{https://github.com/PierreExeter/gym-reacher/blob/master/scripts/DDPG\_reacher.py}
% \item 1) Learning constraint representations/constrainst synthesis
% \item 2) Using dynamics as well to infer constraints better
% \item 3) Literature review in constraint inference
\end{itemize}
